# Supplementary material for: Simulation-based reinforcement learning for real-world autonomous driving
Source: arXiv:1911.12905 source file (2024-04-03)
Supplement: Supplementary file 1 [file appendix.tex]

\appendix

\newpage

\input{network_architecture.tex}

\section{Offline models evaluation}
\label{appendix_offline}

On top of $mae$ metric presented in Section \ref{subsec:offline_models} we have also introduced and evaluated another one: \emph{average F1 score}.
To compute the metric we again process frame by frame human reference drive and compare human action and output of the evaluated model.
We classify requested steering wheel angle into one of three buckets:
left, straight or right, if it is respectively less than $-0.02$ radian, between $-0.02$ and $0.02$ radian or greater than $0.02$ radian.
For each of the buckets, we compute a F1 score between human reference action and the model output. The average of these three values is the final \emph{average F1 score}.
As you can see in Figure \ref{fig:correlations_f1}, this metric also seems to correlate with the model's real-world performance.

\begin{figure}[h]
%\begin{wrapfigure}[21]{c}{0.7\textwidth}
\begin{center}
\includegraphics[width=0.8\linewidth]{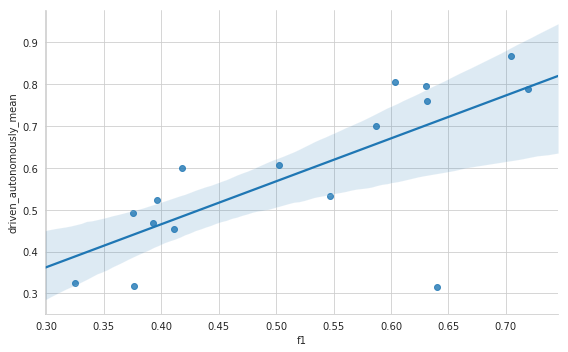}
\caption{Dependence of mean $driven\_autonomously$ metric on their \emph{average F1 score}. Models using waypoitns are not included due to the different action space.}
 \label{fig:correlations_f1}
\end{center}
%\end{wrapfigure}
\end{figure}

\pagebreak
