# Supplementary material for: Simulation-based reinforcement learning for real-world autonomous driving
Source: arXiv:1911.12905 source file (2024-04-03)
Supplement: Supplementary file 2 [file appendix_all_models.tex]

\section{All models}
\label{appendix_all_models}

In the table below we present all models evaluated in the real world.
Their respective performance can be found in Figures \ref{fig:leaderboard_all} and \ref{fig:leaderboard_all_detailed}.

\pagebreak
